# Supplementary material for: WAIC, but Why? Generative Ensembles for Robust Anomaly Detection
Source: arXiv:1810.01392 source file (2019-05-23)
Supplement: Supplementary file 1 [file supplemental_rate.tex]

\section{OoD detection with Rate Terms}

Rate is $\KL ( q_\theta(z|x) \Vert p(z) )$ term in the VAE objective. It represents information loss between encoder distribution and prior over latent code.  Table~\ref{table:supplemental_results_table} shows that rate is a powerful classifier variable in OoD detection. For Fashion MNIST, the same $\beta$-VAE model as the ones for Table 1 of the original paper are used.
