# Supplementary material for: WAIC, but Why? Generative Ensembles for Robust Anomaly Detection
Source: arXiv:1810.01392 source file (2019-05-23)
Supplement: Supplementary file 2 [file supplemental_sensitivity.tex]

\section{Robustness to Perturbations}

\begin{figure}[h]
  \centering
  \includegraphics[width=\linewidth]{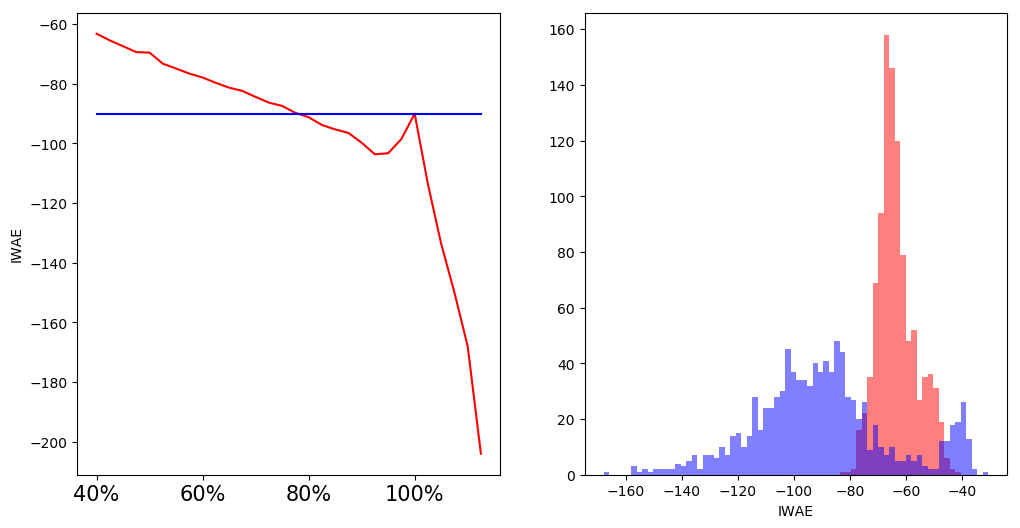}
  \caption{Sensitivity to perturbations. Left: VAE assigns higher IWAE values to scaled-down MNIST (red) than to original MNIST (blue). Starting from a scale of .4, each scale increment corresponds to an image scale by 2.5\%. The red and blue line represent average IWAE over 1000 scaled and original MNIST samples, resp. They intersect at the point where the scale is 100\%. IWAE plummets on scaled-up MNIST. Right: Red histogram corresponds to IWAE on scaled-down MNIST by a scale of .4 and the blue one on original MNIST}
  \label{fig:single_model_failure}
\end{figure}
