# Supplementary material for: WAIC, but Why? Generative Ensembles for Robust Anomaly Detection
Source: arXiv:1810.01392 source file (2019-05-23)
Supplement: Supplementary file 3 [file supplemental_waic.tex]

\section{WAIC}

A principle problem in modelling is attempting to estimate expectations under the true data distribution, as distinct from expectations estimated from the training set.  \emph{Information criteria} offer a means for estimating the difference~\cite{gelman}. In this work we utilize the \emph{Watanabe Akaike Information Criteria}~\cite{watanabe2010asymptotic}, which gives an asymptotically correct estimate.  For completeness, we give a short derivation here following the style and form of \citet{watanabegreen}.
